# Supplementary material for: The Virtual Patch Clamp: Imputing C. elegans Membrane Potentials from Calcium Imaging
Source: arXiv:1907.11075 source file (2019-07-24)
Supplement: Supplementary file 1 [file supplementary.tex]

\documentclass{article}

% if you need to pass options to natbib, use, e.g.:
\PassOptionsToPackage{numbers, sort}{natbib}
% before loading nips_2016
%
% to avoid loading the natbib package, add option nonatbib:
%\usepackagee[nonatbib]{neurips_2019}

\usepackage[preprint]{common/neurips_2019}

% to compile a camera-ready version, add the [final] option, e.g.:
%\usepackage[final]{nips_2016}

\usepackage[utf8]{inputenc} % allow utf-8 input
\usepackage[T1]{fontenc}    % use 8-bit T1 fonts
\usepackage{hyperref}       % hyperlinks
\usepackage{url}            % simple URL typesetting
\usepackage{booktabs}       % professional-quality tables
\usepackage{amsfonts}       % blackboard math symbols
\usepackage{nicefrac}       % compact symbols for 1/2, etc.
\usepackage{microtype}      % microtypography
\usepackage{graphicx}
\usepackage{amsmath}
\usepackage{pdfpages}
\usepackage{makecell}
\usepackage{todonotes}
\usepackage{color}
\usepackage{caption}
\usepackage{tabularx}
\usepackage{cleveref}
\usepackage[numbers]{natbib}
\usepackage{paralist}
\usepackage{relsize}
\usepackage{bbm}
\usepackage{lipsum}  
\usepackage{float}
\usepackage{bibentry}
\usepackage{subfig}

\usepackage{lipsum}
\usepackage{graphicx}
\usepackage{caption}
\usepackage{adjustbox}
\usepackage{pdfpages}
\usepackage{gensymb}
\usepackage{amsfonts}
\usepackage{setspace}
\usepackage{pdflscape}
\usepackage{lscape}
\usepackage{fancyhdr}
\usepackage{relsize}
\usepackage{tabularx}
\usepackage{paralist}

\usepackage{enumitem}
\setitemize{noitemsep,topsep=2pt,parsep=2pt,partopsep=2pt}
\setenumerate{noitemsep,topsep=2pt,parsep=2pt,partopsep=2pt}

\usepackage{bbm}

\usepackage{color}

\usepackage{tikz}
\usetikzlibrary{shapes,arrows}

\usepackage{amsmath}

\usepackage{algorithm}
\usepackage[noend]{algpseudocode}
\makeatletter
\def\BState{\State\hskip-\ALG@thistlm}
\makeatother
\usepackage{multirow}

 % Jan Hlavacek

% Tom's standard shortcuts

%\newcommand{\mG}{\mathcal{G}}

\title{Supplementary Material for: \\ The Virtual Patch Clamp: Imputing \emph{C. elegans} Membrane Potentials from Calcium Imaging}

% The \author macro works with any number of authors. There are two
% commands used to separate the names and addresses of multiple
% authors: \And and \AND.
%
% Using \And between authors leaves it to LaTeX to determine where to
% break the lines. Using \AND forces a line break at that point. So,
% if LaTeX puts 3 of 4 authors names on the first line, and the last
% on the second line, try using \AND instead of \And before the third
% author name.

\author{
Andrew Warrington \\
Department of Engineering Science \\
University of Oxford \\
OX1 3PJ, United Kingdom \\
\texttt{andrew.warrington@keble.ox.ac.uk} \\
\And
Arthur Spencer \\
School of Physiology, \\ Pharmacology \& Neuroscience \\
University of Bristol \\
BS8 1TD, United Kingdom \\
\And
Frank Wood \\
Department of Computer Science \\
University of British Columbia \\
V6T 1Z4, Canada}%

\begin{document}

\setcounter{page}{12}

\maketitle

\newpage
\input{bib}

\end{document}
