# Supplementary material for: The Virtual Patch Clamp: Imputing C. elegans Membrane Potentials from Calcium Imaging
Source: arXiv:1907.11075 source file (2019-07-24)
Supplement: Supplementary file 2 [file supp_preamble.tex]

% if you need to pass options to natbib, use, e.g.:
\PassOptionsToPackage{numbers, sort}{natbib}
% before loading nips_2016
%
% to avoid loading the natbib package, add option nonatbib:
%\usepackagee[nonatbib]{neurips_2019}

\usepackage[preprint]{common/neurips_2019}

% to compile a camera-ready version, add the [final] option, e.g.:
%\usepackage[final]{nips_2016}

\usepackage[utf8]{inputenc} % allow utf-8 input
\usepackage[T1]{fontenc}    % use 8-bit T1 fonts
\usepackage{hyperref}       % hyperlinks
\usepackage{url}            % simple URL typesetting
\usepackage{booktabs}       % professional-quality tables
\usepackage{amsfonts}       % blackboard math symbols
\usepackage{nicefrac}       % compact symbols for 1/2, etc.
\usepackage{microtype}      % microtypography
\usepackage{graphicx}
\usepackage{amsmath}
\usepackage{pdfpages}
\usepackage{makecell}
\usepackage{todonotes}
\usepackage{color}
\usepackage{caption}
\usepackage{tabularx}
\usepackage{cleveref}
\usepackage[numbers]{natbib}
\usepackage{paralist}
\usepackage{relsize}
\usepackage{bbm}
\usepackage{lipsum}  
\usepackage{float}
\usepackage{bibentry}
\usepackage{subfig}

%\usepackage[nocompress]{cite}

\usepackage{lipsum}
\usepackage{graphicx}
%\usepackage{subcaption}
\usepackage{caption}
\usepackage{adjustbox}
\usepackage{pdfpages}
\usepackage{gensymb}
\usepackage{amsfonts}
\usepackage{setspace}
\usepackage{pdflscape}
\usepackage{lscape}
\usepackage{fancyhdr}
\usepackage{relsize}
\usepackage{tabularx}
\usepackage{paralist}

\usepackage{enumitem}
\setitemize{noitemsep,topsep=2pt,parsep=2pt,partopsep=2pt}
\setenumerate{noitemsep,topsep=2pt,parsep=2pt,partopsep=2pt}

\usepackage{bbm}

\usepackage{color}

\usepackage{tikz}
\usetikzlibrary{shapes,arrows}

\usepackage{amsmath}

\usepackage{algorithm}
\usepackage[noend]{algpseudocode}
\makeatletter
\def\BState{\State\hskip-\ALG@thistlm}
\makeatother
\usepackage{multirow}
\DeclareMathOperator*{\argmax}{\arg\!\max}
\DeclareMathOperator*{\argmin}{arg\,min} % Jan Hlavacek

% Tom's standard shortcuts

\newcommand{\mX}{\mathcal{X}}
\newcommand{\mY}{\mathcal{Y}}
\newcommand{\mD}{\mathcal{D}}
%\newcommand{\mG}{\mathcal{G}}
\newcommand{\nx}{_{\mathrm{next}}}
\newcommand{\real}{\mathbb{R}}
\newcommand{\xpos}{\tilde{\mathbf{x}}}
\newcommand{\xb}{\mathbf{x}}
\newcommand{\yb}{\mathbf{y}}
\newcommand{\zb}{\mathbf{z}}
\newcommand{\hb}{\mathbf{h}}
\newcommand{\hx}{h\left(\xb,\zb\right)}
\newcommand{\bc}{\left(\cdot\right)}
\newcommand{\bcc}{\left(\cdot\right)}
\newcommand{\mM}{\mathcal{M}}
\newcommand{\tx}{\texttt{x}}
\newcommand{\ty}{\texttt{y}}
\newcommand{\tz}{\texttt{z}}
\newcommand{\tb}{\texttt{b}}
\newcommand{\ft}{f\left(\theta\right)}
\newcommand{\hth}{\hat{\theta}}
\newcommand{\hu}{\hat{U}}
\newcommand{\hy}{\hat{y}}
\newcommand{\hY}{\hat{Y}}
\newcommand{\hZ}{\hat{Z}}
\newcommand{\hup}{\hat{\upsilon}}
\newcommand{\hsig}{\hat{\sigma}}


\newcommand{\cef}{\emph{Caenorhabditis elegans}}
\newcommand{\ce}{\emph{C. elegans}}
\newcommand{\kl}{\textsc{KL}}
\newcommand{\elbo}{\textsc{ELBO}}



\newcommand{\aw}[1]{\textcolor{magenta}{[AW: #1]}}
\newcommand{\as}[1]{\textcolor{red}{[AS: #1]}}
\newcommand{\fw}[1]{\textcolor{green}{[FW: #1]}}



\title{Supplementary Material for: \\ The Virtual Patch Clamp: Imputing \emph{C. elegans} Membrane Potentials from Calcium Imaging}

% The \author macro works with any number of authors. There are two
% commands used to separate the names and addresses of multiple
% authors: \And and \AND.
%
% Using \And between authors leaves it to LaTeX to determine where to
% break the lines. Using \AND forces a line break at that point. So,
% if LaTeX puts 3 of 4 authors names on the first line, and the last
% on the second line, try using \AND instead of \And before the third
% author name.

\author{
Andrew Warrington \\
Department of Engineering Science \\
University of Oxford \\
OX1 3PJ, United Kingdom \\
\texttt{andrew.warrington@keble.ox.ac.uk} \\
\And
Arthur Spencer \\
School of Physiology, \\ Pharmacology \& Neuroscience \\
University of Bristol \\
BS8 1TD, United Kingdom \\
\And
Frank Wood \\
Department of Computer Science \\
University of British Columbia \\
V6T 1Z4, Canada}%
